# Supplementary material for: Trident: Efficient 4PC Framework for Privacy Preserving Machine Learning
Source: arXiv:1912.02631 source file (2021-06-08)
Supplement: Supplementary file 1 [file Appendix_BenchSemiCost.tex]

In this section, .... ABY3 is used to denoted semi-honest version of ABY3
%--------------------------------
\subsection{Secure Training}
%--------------------------------
\commentAJ{Feature Size 784 and batch size 128. Giving the number of iterations as benchmark parameter.

%--------------------------------
\subsection{Secure Prediction}
%--------------------------------
\commentAJ{Feature Size 784 and batch of 100. Giving the throughput as benchmark parameter. For preprocessing, add details verbally. Argument similar to training}
