# Supplementary material for: Trident: Efficient 4PC Framework for Privacy Preserving Machine Learning
Source: arXiv:1912.02631 source file (2021-06-08)
Supplement: Supplementary file 2 [file Appendix_GordonComp.tex]

In this section, we compare our 4PC protocol with that of Gordon et al.~\cite{GordonR018} in terms of practical efficiency. \commentAJ{Add details here...Use AES circuit for benchmarking. See the table for what details we are giving. We will be giving what percent of total runtime and communication each party is having when compared with the total value}
