# Supplementary material for: Trident: Efficient 4PC Framework for Privacy Preserving Machine Learning
Source: arXiv:1912.02631 source file (2021-06-08)
Supplement: Supplementary file 3 [file Appendix_PrivML.tex]

In this section, we will introduce the necessary background for the following machine learning algorithms used by our protocols:
